# Supplementary material for: HyperDreamer: Hyper-Realistic 3D Content Generation and Editing from a Single Image
Source: arXiv:2312.04543 source file (2023-12-07)
Supplement: Supplementary file 1 [file supp.tex]

% \newpage
\appendix
\setcounter{table}{0}
\setcounter{figure}{0}

\section{Additional Implementation Details}

\subsection{Interactive Editing}

In the editing first stage, we found the selection of the location and number of points will affect the segmentation results significantly When sampling the point prompts from cache. Simply inputting all the point prompts in each view may cause GPU memory explosion, and random sampling will also lead to unsatisfactory final results. Therefore, based on the consideration of computing resource consumption and segmentation accuracy, we adopted the scheme of patch sampling. In our method, from $v_t$ view, we split the $Q_{mask}^{t-1}$ and $Q_{negmask}^{t-1}$ to 25 $\times$ 25 and 5 $\times$ 5 respectively, then sampling the points within each patch,  which ensures the geometric uniformity of the sampling to some extent. But if the number of point prompts in a patch is less than a threshold $\theta$ we will not sample in there, which reduces the impact of out-lie points on the results. 

\subsection{Material Modeling}
we assume that regions with the same semantic label usually share alike materials. Similar to the albedo learning, we maintain two semantic-aware learnable vectors for roughness $R_s$ and specular $S_s$. The dimensions of them are $N_s \times 1$ and $N_s \times 3$, respectively. We adopt a white specular color assumption and enforce channel consistency in $R_s$. We also incorporate two MLP-based predictors to predict offsets for roughness and specular based on $R_s$ and $S_s$ to enable a more flexible and fine-grained material modeling.

We leverage the specular term $I_{spec}$ predicted by~\cite{wimbauer2022derendering} and the semantic segmentation to initialize $S_s$. In addition, we use an off-shelf method to generate a normal map, which allows for an improved realism and increased details.
For our online semantic segmentation approach, we initiate the process by generating over-segmentation results through the employment of SAM, which yields a set of fine-grained semantic segments. These segments are then subjected to feature extraction, encompassing attributes such as RGB color, HSV color, and SAM-generated features. The resulting features are averaged within each segment, serving as the foundational evidence for subsequent clustering.
Primarily, RGB colors are often sufficient for a wide array of scenarios. With this foundation in place, our methodology commences by targeting the segment with the smallest area, systematically progressing through to the largest. At this stage, a novel segment is confronted with two possibilities: it either integrates into pre-existing segments provided its feature similarity surpasses a predefined threshold, or it is designated as a distinct semantic label.
This iterative process ensures the gradual amalgamation of the over-segmented outcomes, effectively yielding succinct and mutually exclusive semantic regions.

For the design of semantic-aware roughness and specular, we can utilize results from pre-trained de-rendering methods~\cite{sang2020single,wimbauer2022derendering} for initialization. For SVBRDF-based models, an averaged value within a semantic label can serve as the initial value. While for those who model a global specular strength and intensity, we can leverage the predicted specular reflectance image $I_{spec}$ and the semantic segmentation to initialize $S_s$ with a relative value. Specifically, we directly aggregate the per-pixel specular reflectance values within each semantic label. The relative specular initialization is then calculated as the difference between the average top 20\% and average bottom 20\% of these values. The optimization is relatively robust to the initialization material settings, which mainly affects the optimization at the earlier stages.

\subsection{Super Resolution Module}
In the refining stage, we employ our Super Resolution Module to enhance the texture quality. To ensure comprehensive coverage of the object and minimize overlap, we typically select left, right, and back views as pseudo-reference views. Subsequently, we generate 3-4 images per view directly using Zero-1-to-3~\cite{liu2023zero123}. We further utilize the Stable Diffusion Upscaler~\cite{rombach2021highresolution}, a text-guided latent upscaling diffusion model, to upscale these images by four times. During training, we randomly sample one pseudo-reference image and its corresponding pseudo-reference view every five steps. We calculate the perceptual loss to guide the training process and optimize the model's performance.

\section{Additional Related Works in Details}
\label{sec:related_works}
\subsection{Text-guided 3D Generation.}
The text-guided 3D generation has gained significant attention following the remarkable success of text-to-image generation methods. Existing approaches in this area can be categorized into two main groups: inference-based methods~\cite{sanghi2021clip, nichol2022pointe, jun2023shap-e} and optimization-based methods~\cite{wang2022sjc, jain2021dreamfields, poole2022dreamfusion, lin2023magic3d, chen2023fantasia3d, lee2022understanding, metzer2022latent}.

Inference-based methods offer the advantage of quickly generating 3D assets by avoiding computationally expensive optimization procedures. However, their reliance on 3D data limits their ability to generate diverse 3D objects and produce high-quality results.

In contrast, optimization-based methods eliminate the need for 3D data. These methods achieve text-to-3D generation through two critical components: differentiable 3D representations and large pretrained 2D models. By rendering randomly initialized 3D models into 2D images, these methods leverage pretrained 2D models to provide supervision signals and update the parameters of the 3D representations.
Dream Fields~\cite{jain2021dreamfields} employed the text-image model CLIP~\cite{radford2021learning} to optimize NeRFs~\cite{mildenhall2020nerf} by aligning the text and image embeddings.
Building on the same principle, DreamFusion~\cite{poole2022dreamfusion} replaced CLIP with diffusion models and devised an SDS loss to distill knowledge from the denoising procedures.
Magic3D~\cite{lin2023magic3d} further enhanced generation performance in terms of synthesis quality and running time by employing a coarse-to-fine framework and using meshes as the 3D representation in the second stage, enabling fast and high-resolution rendering.
Fantasia3D~\cite{chen2023fantasia3d} introduced the spatially varying bidirectional reflectance distribution function (SVBRDF)~\cite{aittala2013practical} into this task, enabling the disentanglement of geometry and appearance. By utilizing a more complex and physically accurate shading model, Fantasia3D achieved the generation of photorealistic 3D assets.

In contrast to the aforementioned methods, our approach distinguishes itself by utilizing a single image as the guided condition instead of text. This choice of using images provides more detailed and specific information, making it more suitable for customized design purposes.

\subsection{Single-image Reconstruction.}
Reconstructing 3D models from a single image has been a long existing topic. Traditional methods heavily rely on 3D datasets for training, which limits their generalization capabilities. Some approaches require training category-specific models from scratch for each object class~\cite{choy20163d, tulsiani2017multi, melaskyriazi2023projection, gu2023nerfdiff, pavllo2023shape}. Others aim to handle multi-class or more general scenarios~\cite{vasudev2022ss3d, wu2023multiview, huang2023shapeclipper}. More recently, Point-E~\cite{nichol2022pointe} and Shap-E~\cite{jun2023shap-e} leverage large 3D datasets, allowing for the generation of complex and diverse 3D assets.

Our focus is on reconstruction methods that leverage 2D priors to reduce the reliance on extensive 3D training datasets. These methods adopt similar principles to text-guided 3D generation but benefit from the rich details present in the reference image by incorporating reconstruction objectives at the frontal view~\cite{Xu_2022_neuralLift, melaskyriazi2023realfusion, tang2023make, deng2022nerdi}.
Realfusion~\cite{melaskyriazi2023realfusion} employs single-image textual inversion to bridge the gap between the reference image and text-conditioned guidance. However, the textural inversion process is time-consuming, and the use of NeRF representation limits the rendering resolution and quality. Make-it-3D~\cite{tang2023make} employs a two-stage optimization pipeline: the first stage optimizes a NeRF model; the second stage transforms the coarse model into textured point clouds and enhances realism with diffusion priors while leveraging high-quality textures from the reference image. 

Most recently, Zero-1-to-3~\cite{liu2023zero123} proposes a method to control camera perspective in diffusion models~\cite{rombach2021highresolution}, enabling novel view synthesis from a single image. It has also been applied to single-image 3D reconstruction by incorporating it with SJC~\cite{wang2022sjc}. In our work, we also utilize Zero-1-to-3 as the guidance model and extend the prior body of work by incorporating a novel material estimation method into the reconstruction procedure.

\subsection{Material and Illumination Estimation}
%

% nerf-based rerendering / relighting (given multi-view images)
% (Extracting Triangular 3D Models, Materials, and Lighting From Images)

The task of estimating material and illumination has long been a focus in both computer vision and computer graphics. Recent reconstruction methods~\cite{munkberg2022extracting} have aimed to learn disentangled 3D representations by separately modeling and learning geometry, material, and illumination conditions. The objective is to achieve improved performance and direct integration into modern rendering engines. However, these methods may not be universally applicable as they rely on multi-view images.
% decomposition from a single image 
Another line of research directly estimates material and lighting from a single image~\cite{wimbauer2022derendering, sang2020single, physg2021}. Give the highly ill-posed nature of this decomposition problem, a spatially varying parameterization often leads to degenerate results. 
Some approaches have addressed this issue by assuming a monochrome specular property as a strong regularization for the neural network. However, this assumption is overly simplistic and insufficient for modeling complex objects.

In this work, we propose a more plausible assumption: materials within the same semantic class share identical specular properties. By making this assumption, we enable the modeling of objects with different materials while preventing the neural network from generating degenerate solutions. This semantic constraint distinguishes our method from Fantasia3D, which learns global roughness and metallic distributions that may not always align with realistic material properties.

% In this work, we aim to ... (discuss the difference between us and tango, fantasia3d) 
% Learning a single global material property is insufficient for modeling complex objects, while implementing a spatially varying parameterization is often too under-constrained, making it difficult to formulating a reasonable distribution globally. We ...

% \begin{figure}
% 	\centering
% 	\includegraphics[width=1.0\linewidth]{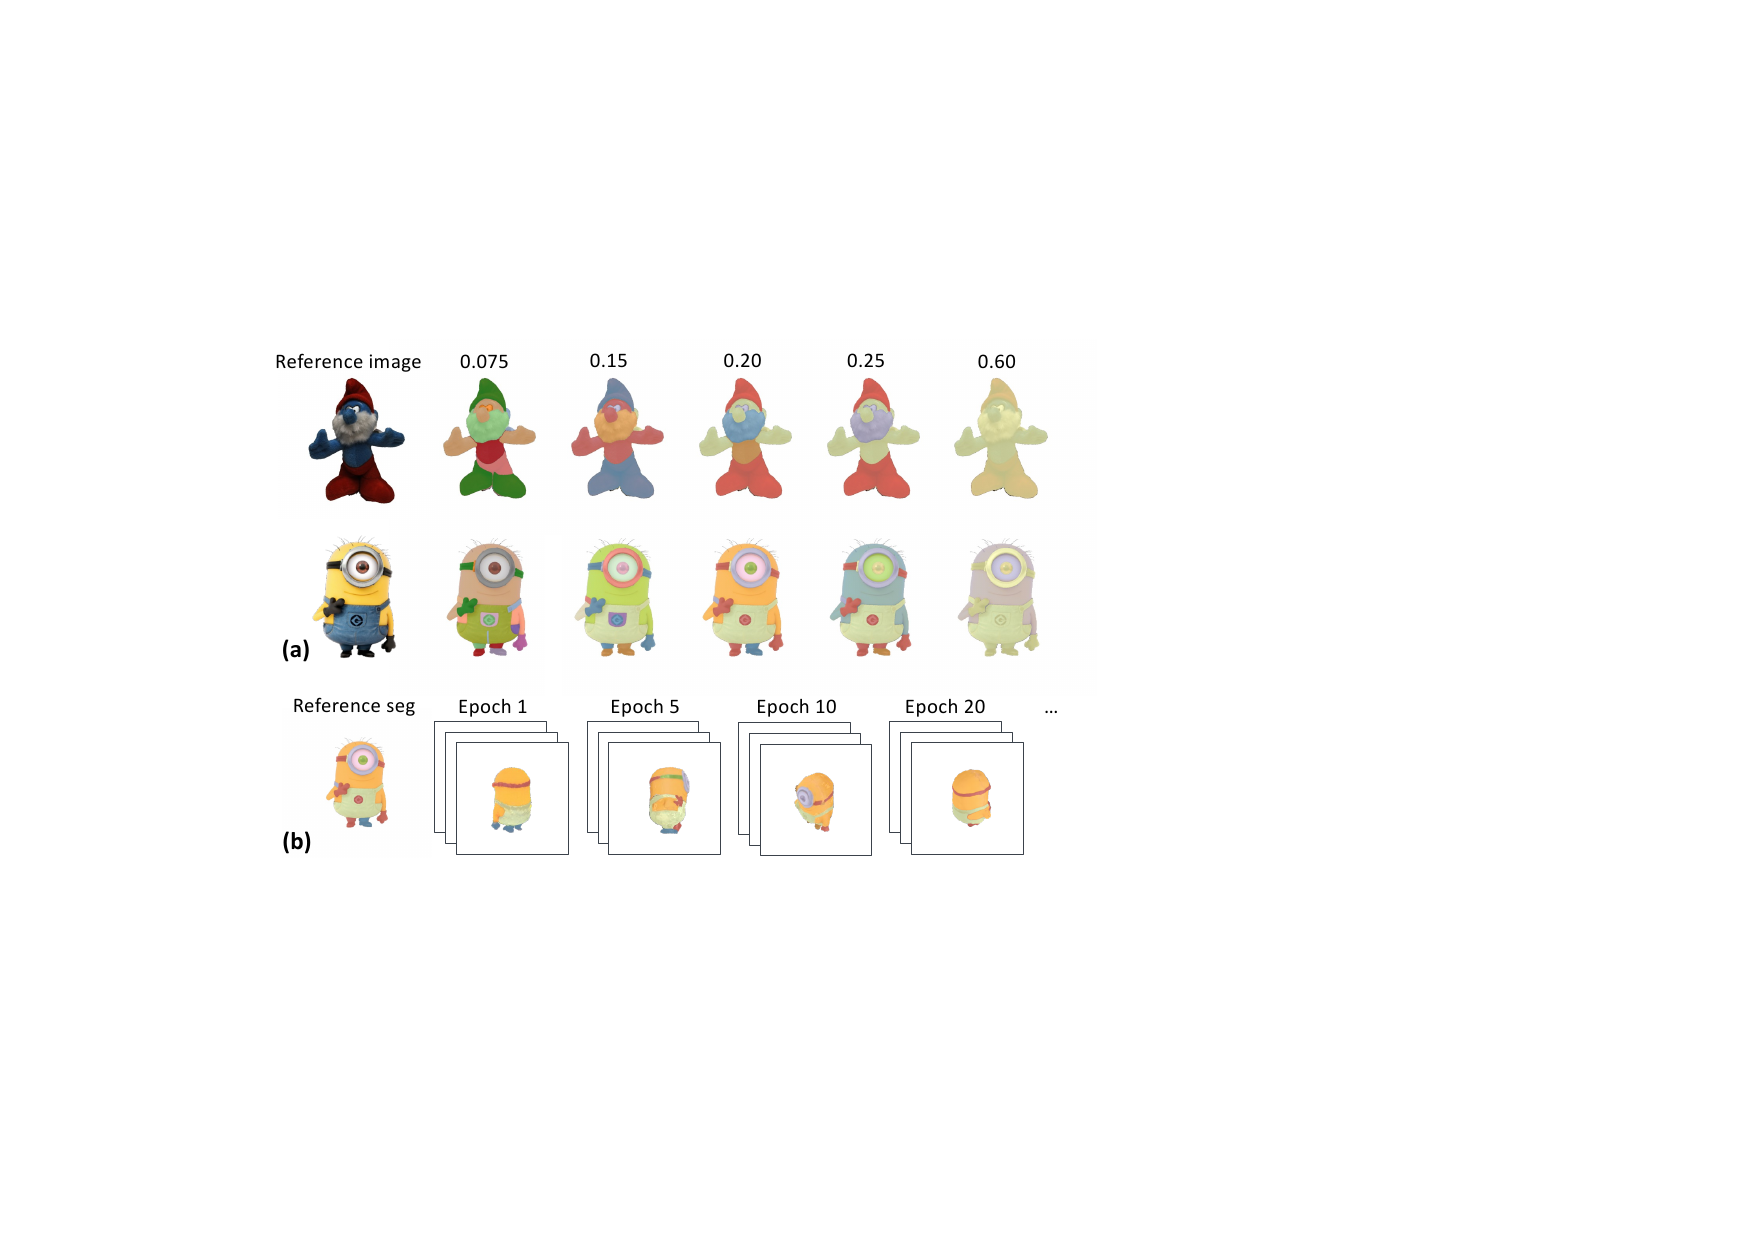}
%         \setlength{\abovecaptionskip}{-3mm}
% 	\caption{\small
%         \textbf{Ablation on online segmentation.}  \textbf{(a)} thresholds spanning from 0.15 to 0.3 consistently yield plausible segmentation clustering. Deviating to larger or smaller values results in under-segmentation or excessive over-segmentation, respectively. \textbf{(b)} the identical threshold value is employed for generating pseudo labels for novel views during the training process.
% 	}
% 	\label{fig:segmentation_abl}
%        \vspace{-15pt}
% \end{figure}

\begin{figure}
	\centering
	\includegraphics[width=1.0\linewidth]{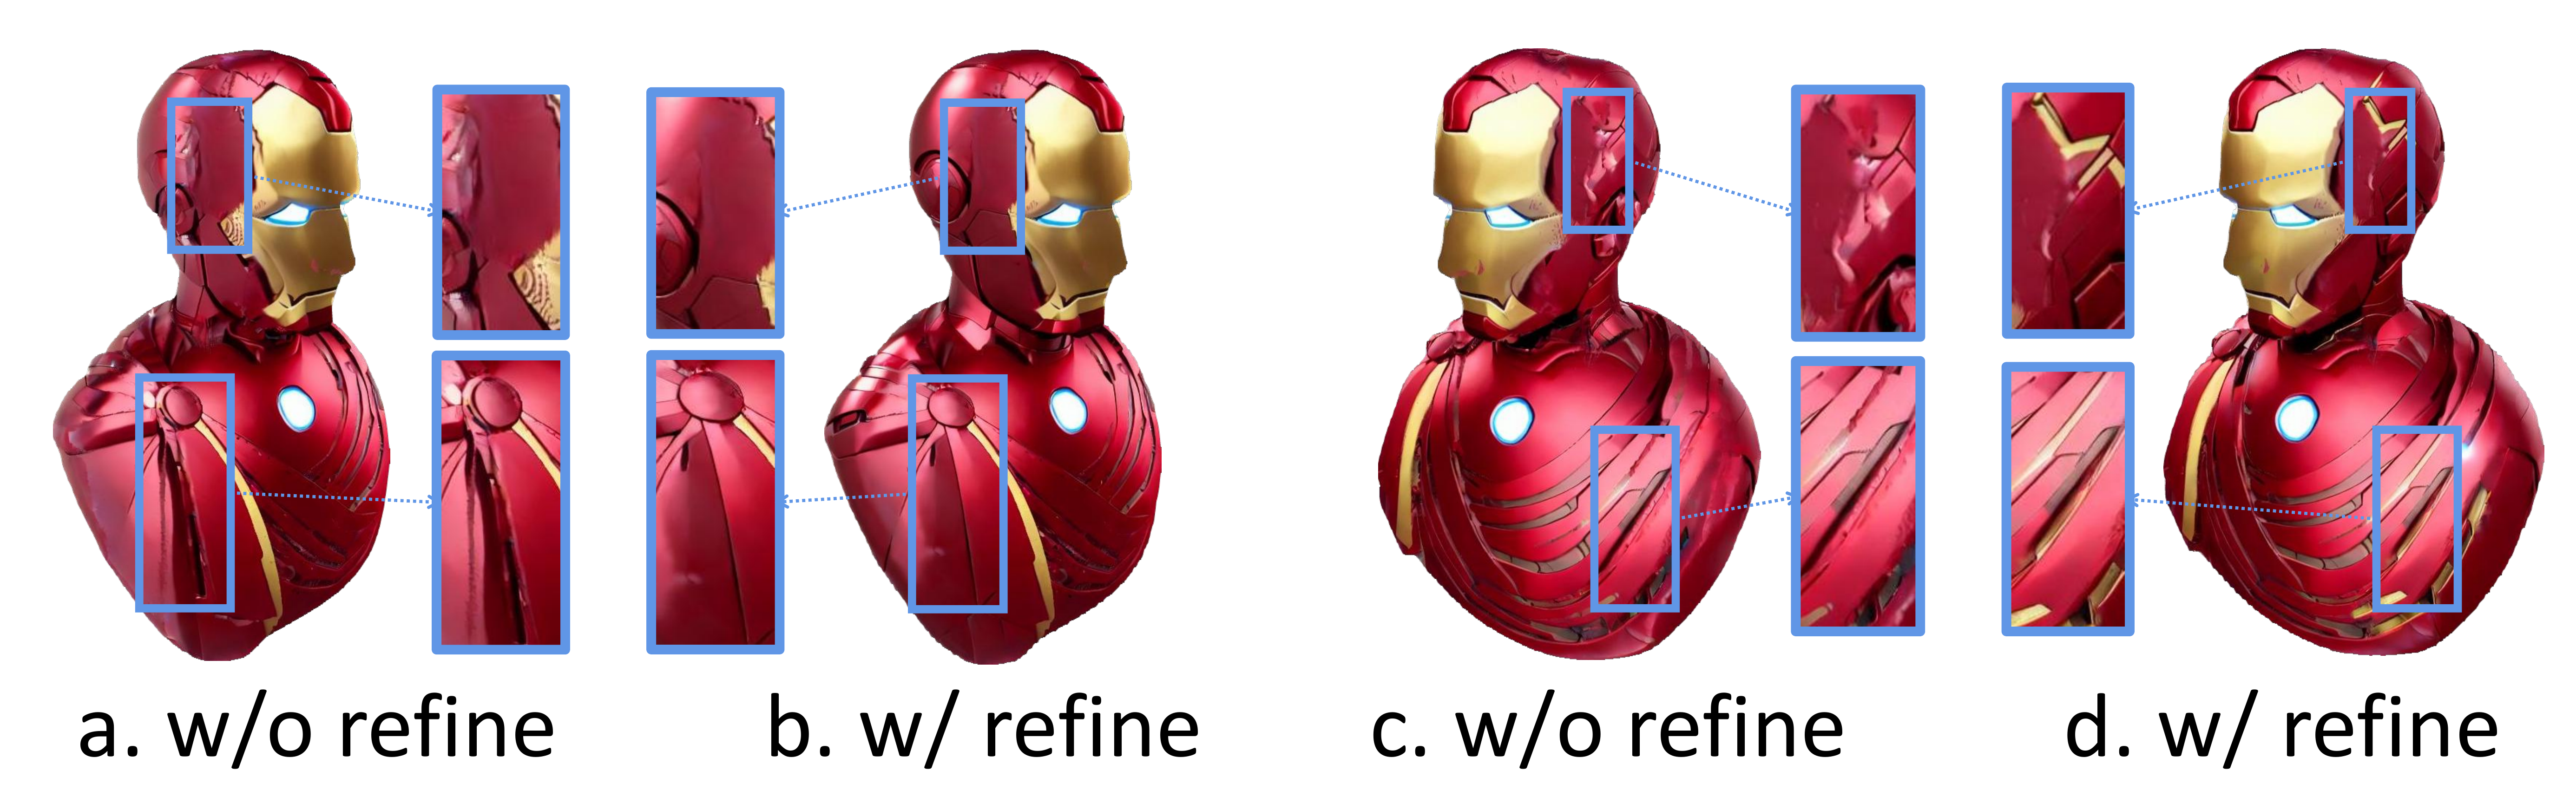}
        \setlength{\abovecaptionskip}{-3mm}
	\caption{\small
        \textbf{Ablation on the refine stage of texture editing.} The proposed refine technique can effectively improve the texture quality and maintain consistency by inpainting the junction regions.
	}
	\label{fig:refine_ablation}
       \vspace{-15pt}
\end{figure}

\begin{figure}[t]
	\centering
	\includegraphics[width=1.0\linewidth]{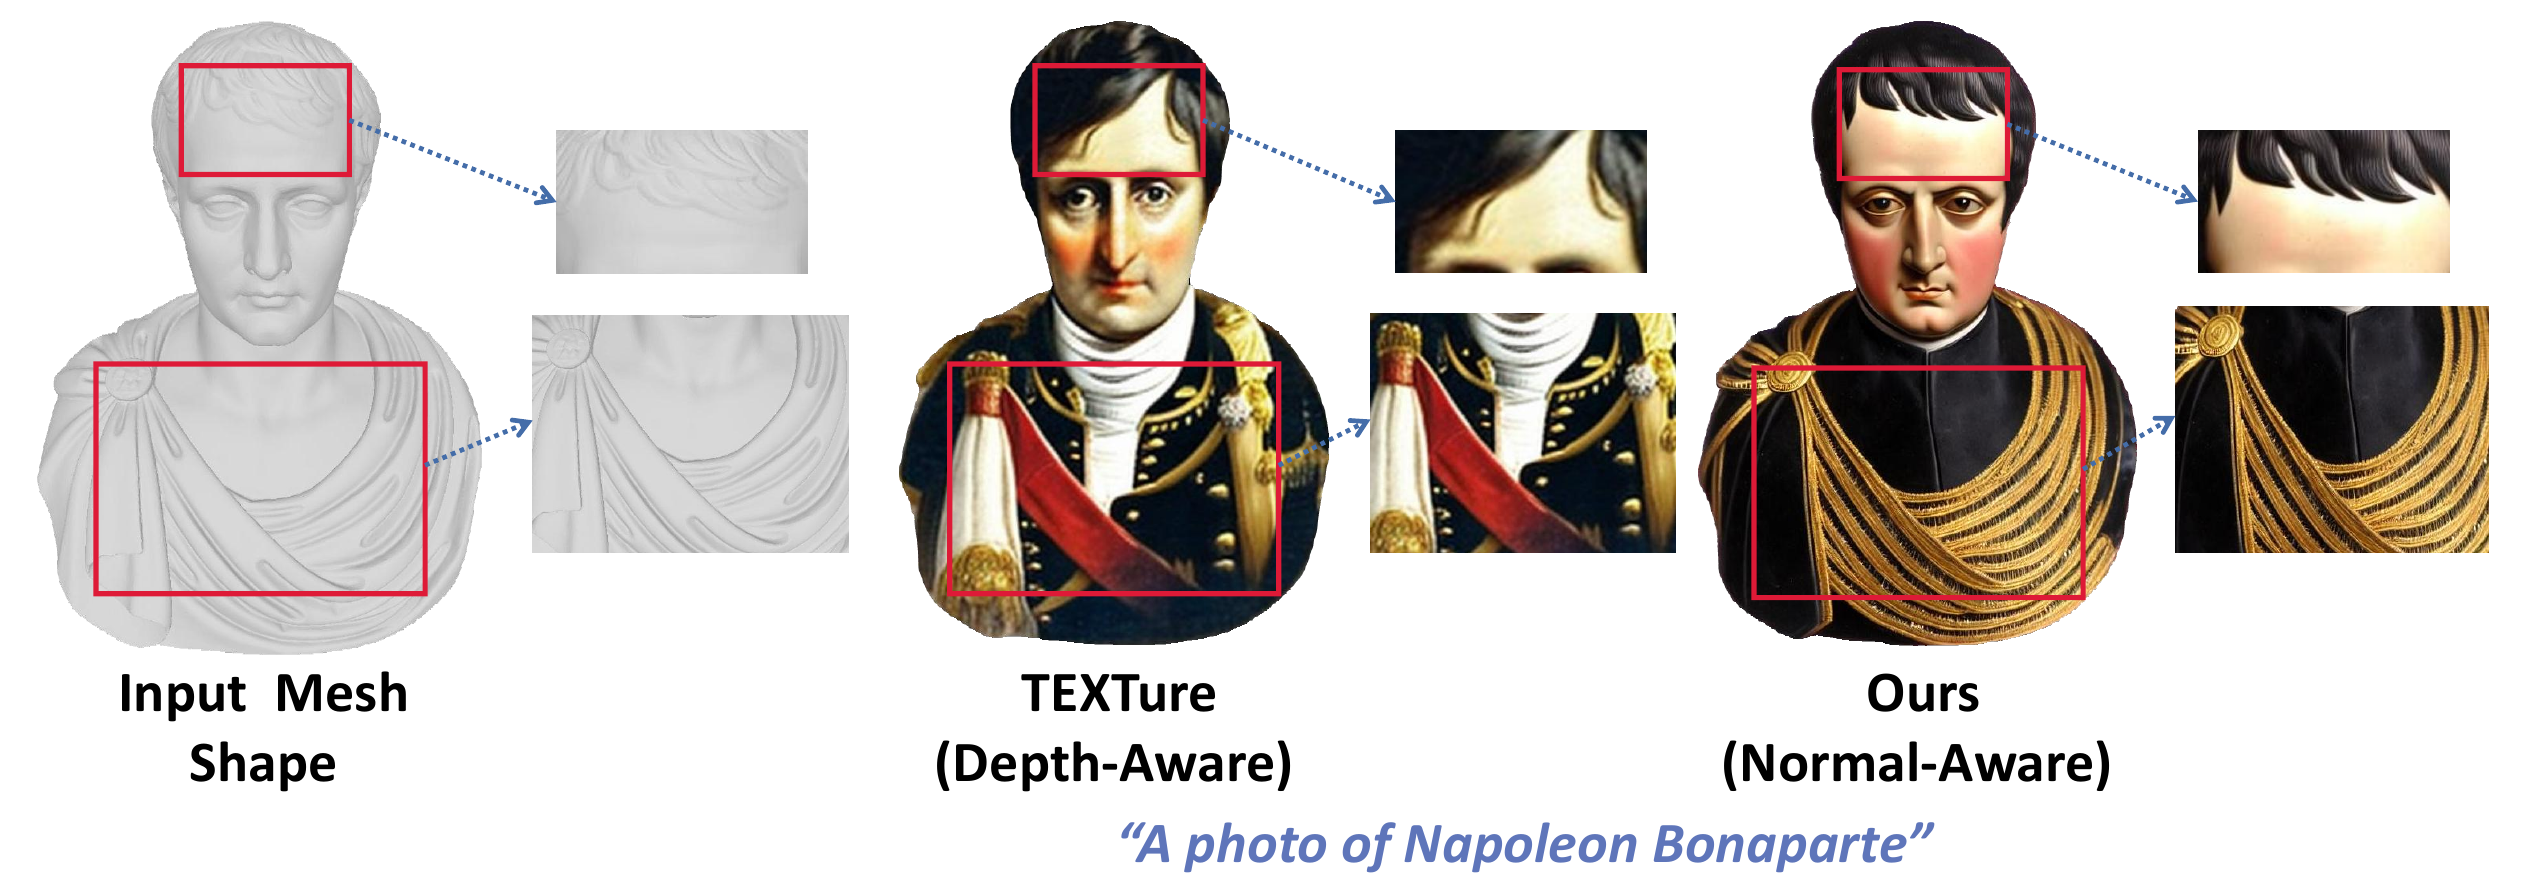}
        \setlength{\abovecaptionskip}{-3mm}
	\caption{\textbf{Ablation on the improved Normal-Aware Model.} Compared to TEXTure based on depth-aware model, in the example of "A photo of Napoleon Bonaparte", whether it is the orientation of the bangs or the clothes at the chest, ours are closer to the shape of the original mesh.  
	}
	\label{fig:normal_aware_ablation}
        \vspace{-5pt}
\end{figure}

%
% \begin{figure*}[t]
% 	\centering
% 	\includegraphics[width=1.0\linewidth]{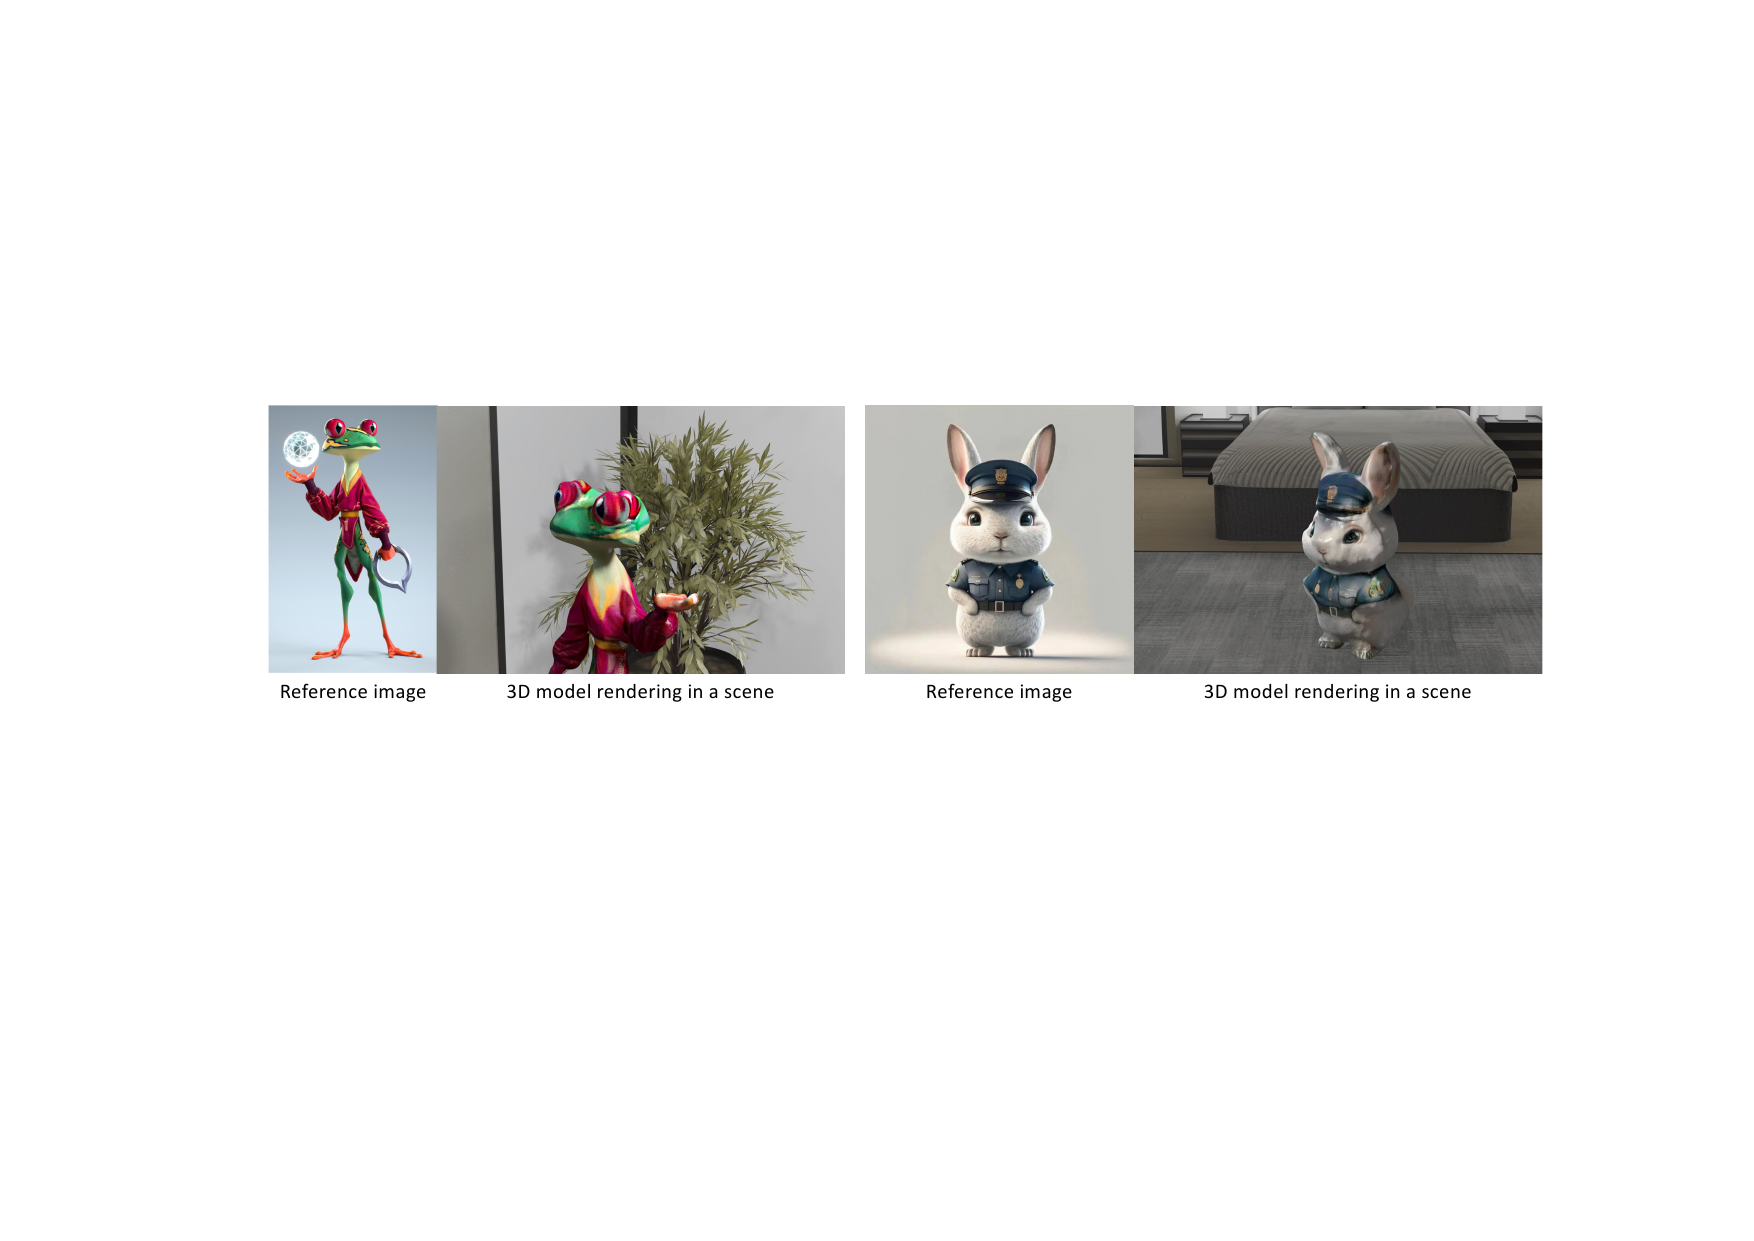}
%         \setlength{\abovecaptionskip}{-3mm}
% 	\caption{\textbf{Rendering results in blender.} We use a custom environment in blender and render the textured mesh with materials. 
% 	}
% 	\label{fig:blender}
% \end{figure*}

\subsection{Text-guided 3D Editing.}
%

% traditional methods
% need a survey

% morden methods
% text2mesh, latent-paint, tango (mention the weakness of its material generation), texturepaper, the one that looks basically the same as texturepaper
Recently, text guided image processing has experienced a rapid development, both in the generation of high-quality images and in the diverse editing of images. However, the existing text-based methods for operating on 3D objects are relatively less common. Text2Mesh~\cite{michel2022text2mesh} proposes a neural style field, which uses CLIP to guide and optimize the initial mesh based on text. TANGO~\cite{chen2022tango} follows a similar scheme and uses a bidirectional reflectance distribution function to optimize the appearance. Also it can obtain the material of the bare mesh under the text description in the meantime, but there is still a gap from the actual use due to accuracy and other reasons. Latent-paint~\cite{metzer2022latent} is a texture generation technique that uses Score-Distillation~\cite{poole2022dreamfusion} to texture on the original mesh, which suffers from poor clarity due to its weak sensitivity to high-frequency details. Instruct 3D-3D~\cite{kamata2023instruct} can convert a given 3D scene to another scene based on text description. Vox-E~\cite{sella2023vox} proposes a new volumetric regularization loss that can directly manipulate object in 3D space. TEXTure~\cite{richardson2023texture} leverages an improved depth-to-image diffusion process and applies an iterative scheme that paints a 3D model from different viewpoints. In addition, it provides scribble-based editing that users can paint in a specific render view and then project-back to the mesh to edit texture maps. Although these methods have their own characteristics in editing 3D objects, none of them can achieve text-guided editing in a given 3D object limited to a local area in 3D space.

In our work, we propose an interactive editing method that users can edit textures based on text guidance in selected 3D regions with a few simple clicks. In the same way, this also supports directly selecting the entire object for global editing to transform style.

\section{Additional Experimental results}
%

% \mdf{
% \subsection{Ablation on online semantic segmentation}
% The most critical hyper-parameter for the online segmentation process is the threshold for clustering. Experimental results reveal that a broad spectrum of thresholding values ranging from 0.15 to 0.3 facilitates effective clustering,, as shown in Figure~\ref{fig:segmentation_abl} (a). The same threshold holds when we define pseudo labels on novel view images along with the optimization to train the globally consistent mesh segmentation branch.   
% }

\subsection{Analysis on the texturing refine stage}
As shown in Figure~\ref{fig:refine_ablation}, via refining the junction of adjacent view, some blurry artifacts and projection seams can be eliminated effectively, stitching the textures more naturally and smoothly when texturing.

\begin{figure}
	\centering
	\includegraphics[width=1.0\linewidth]{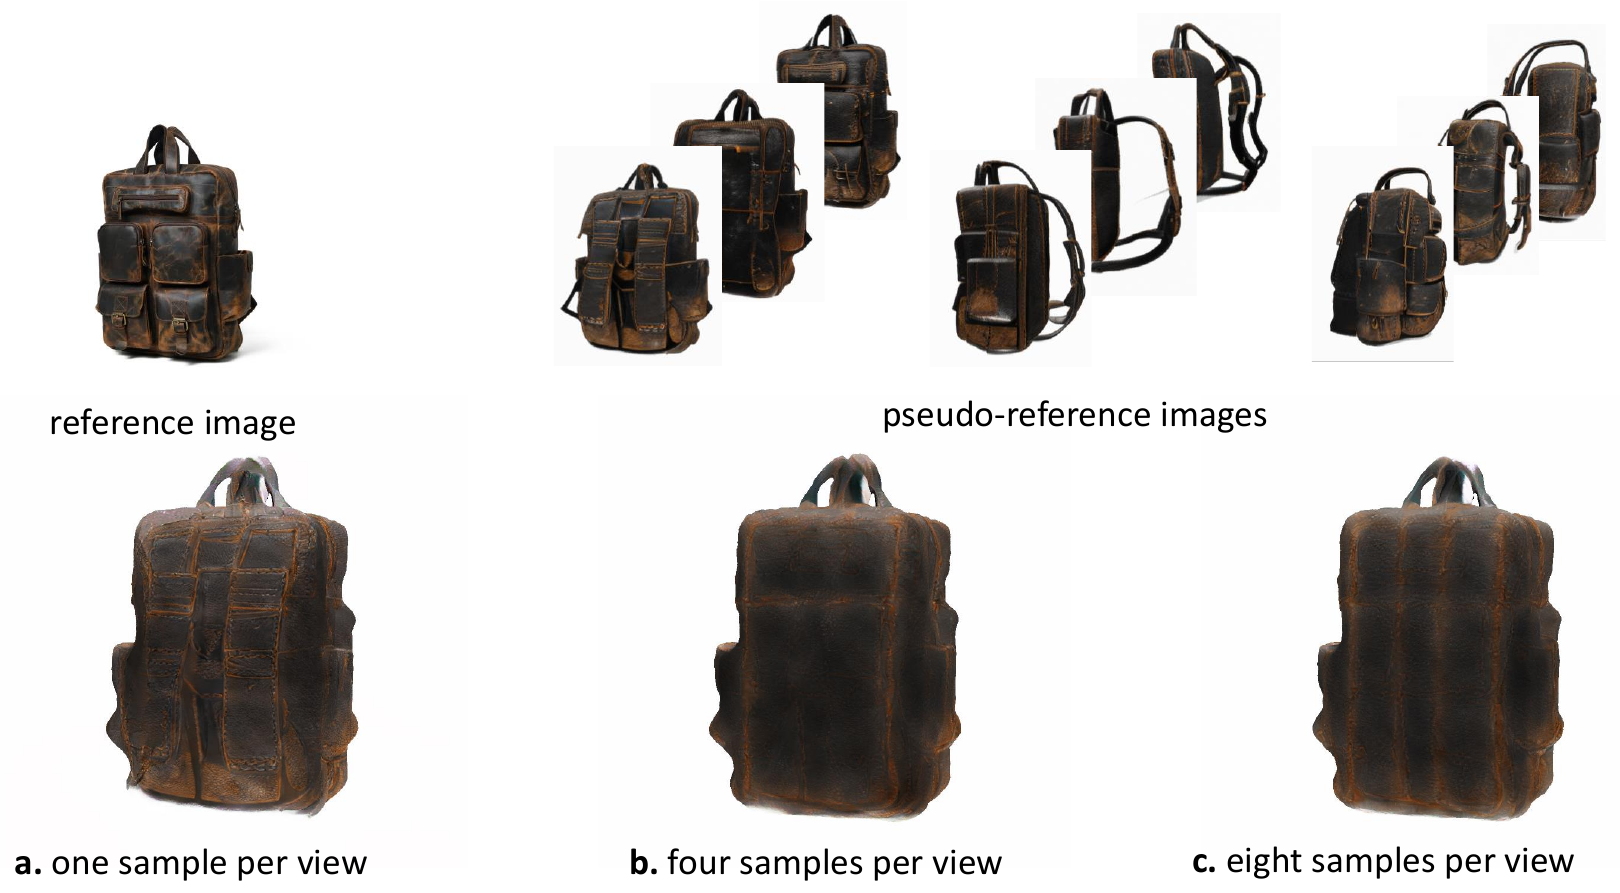}
        \setlength{\abovecaptionskip}{-3mm}
	\caption{\textbf{Ablation study of SR Module.} Increase the number of samples per pseudo-reference view can effectively mitigated the misalignment issue.}
	\label{fig:sr_ab}
        \vspace{-5pt}
\end{figure}

% Table generated by Excel2LaTeX from sheet 'Sheet1'
\begin{table}[t]
  \centering
  \caption{\textbf{Geometry evaluation on the DTU dataset.} $CD_{full}$ denotes the standard Chamfer Distance; $CD_{partial}$ quantifies the distance from the partial ground truth to the complete 3D output only.}
    \small
    \resizebox{.48\textwidth}{!} {
    \begin{tabular}{l|ccccc}
    \toprule
    
    Method & \multicolumn{1}{l}{Shap-E} & \multicolumn{1}{l}{Neurallift-360} & \multicolumn{1}{l}{Realfusion} & \multicolumn{1}{l}{Zero-1-to-3} & \multicolumn{1}{l}{Ours} \\
    \midrule
    $CD_{full} \downarrow$ & 0.039 & 0.045 & 0.037 & 0.038 & \textbf{0.035} \\
    $CD_{partial} \downarrow$ & 0.036 & 0.042 & \textbf{0.032} & 0.036 & \textbf{0.032} \\
    \bottomrule
    
    \end{tabular}%
    }
  \label{tab:dtu_geo}%
\end{table}%

\subsection{Analysis on the Normal-Aware Model}
To verify the effectiveness of key module in our text-guided texture synthesis method , we conduct another ablation study in Figure~\ref{fig:normal_aware_ablation}. We can find that the normal-aware diffusion model is very important for generating textures that fit the geometric details of the mesh. Especially, compared to the depth-aware model with a certain ability to generate consistency, we found that ours is more in line with the original shape and has higher clarity, whether in the bangs or the chest of napoleon.

\subsection{Analysis on the Super Resolution Module}
To assess the impact of the number of samples per pseudo-reference view, we trained \ourmodel~ under different number of samples per view. The results of these experiments are presented in Figure~\ref{fig:sr_ab}.

When only one image provided under a view, it can potentially mislead the generation process due to imperfect alignment with the generated 3D model. 
This can lead to artifacts or distortions in the generated output, as illustrated in Figure~\ref{fig:sr_ab}-a, where two "straps" appear in the back view despite the back being relatively flat in terms of its geometry. However, increasing the number of pseudo-reference images can effectively alleviate this issue. In Figure~\ref{fig:sr_ab}-b, we can see that when more pseudo-reference images are available, the model tends to learn the material characteristics from these images rather than relying on specific structural details. We observed that four images per view can handle most misalignment problems without incurring excessive computational resources.

\subsection{Geometry Evaluation}
We evaluate the geometry accuracy of the generated 3D models on the DTU~\cite{jensen2014large} dataset. We follow recent advances on 3D neural surface reconstruction~\cite{yariv2020multiview,wang2021neus,wu2022voxurf} and evaluate on a subset of 15 scenes. To address the misalignment in coordinate systems between different methods and the DTU ground truth, We manually align the generated models with the 3D ground truth via Blender before calculating the Chamfer Distance (CD). 
It's worth noting that the ground truth DTU point clouds typically capture only partial aspects of geometry, predominantly from a frontal viewpoint. Given this inherent limitation, a standard CD measurement, denoted as $CD_{full}$ might not provide a comprehensive assessment. We thus introduce $CD_{partial}$, which quantifies the distance from the ground truth to the complete 3D output only. The results are shown in Table~\ref{tab:dtu_geo}, where our method demonstrates higher geometry accuracy on both metrics.

% %
% \section{Rendering in Blender}
% %
% We load the generated models with albedo, roughness, and specular maps into a custom environment in Blender and test their usage in modern rendering engines. The generated model shows the potential to be practical in real applications.
\begin{figure}[t]
	\centering
	\includegraphics[width=1.0\linewidth]{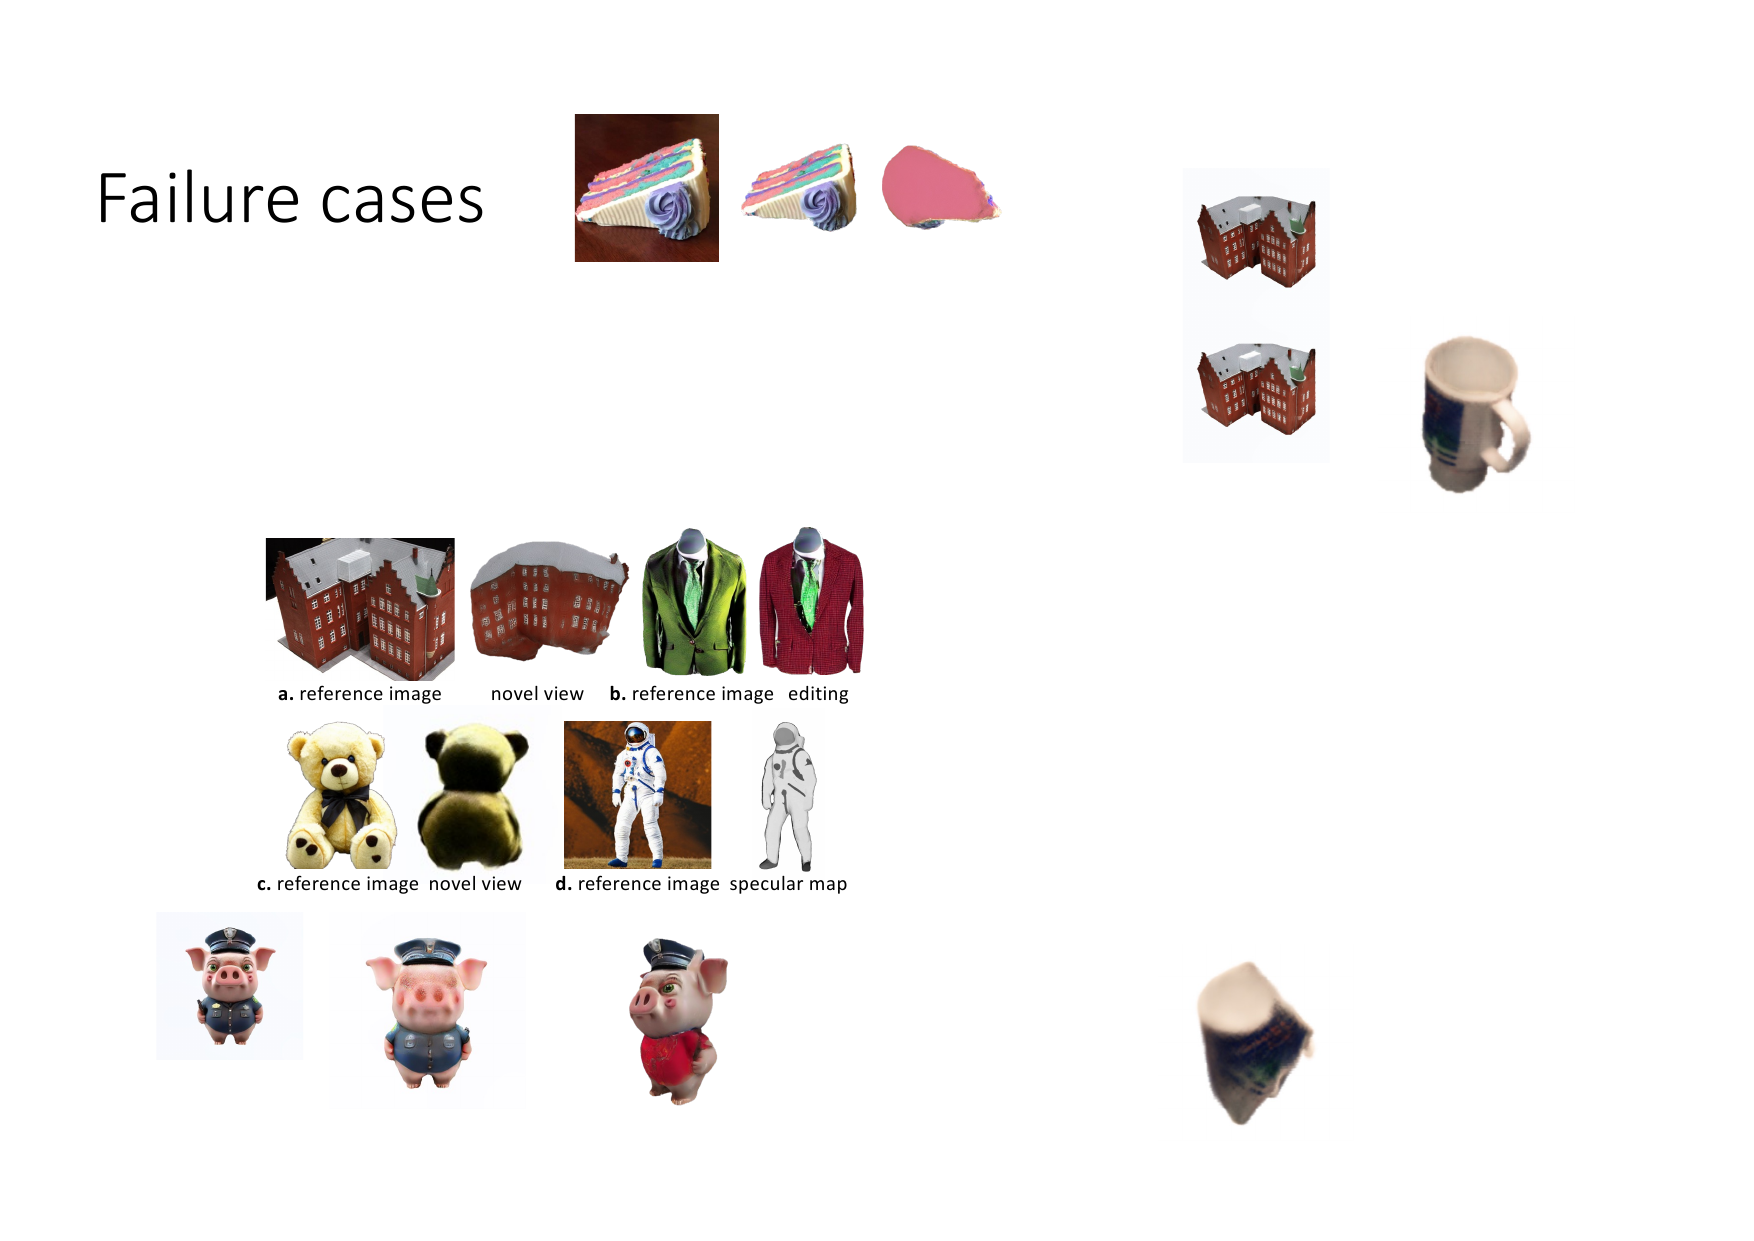}
        \setlength{\abovecaptionskip}{-3mm}
	\caption{\textbf{Failure cases.} We show indicative instances of failure pertaining to geometry (a), editing (b), and material (c)(d).
	}
	\label{fig:failure_case}
        \vspace{-5pt}
\end{figure}

\subsection{Uncurated Results}
In this section, we present some uncurated results of \ourmodel~. We have gathered samples from the official repository of Make-It-3D~\cite{tang2023make}, the DTU dataset~\cite{aanaes2016large} and the Internet, \textbf{without any cherry-picking}.
% We include \textbf{all} the samples collected from official repositories of RealFusion~\cite{melaskyriazi2023realfusion}, Zero-1-to-3~\cite{liu2023zero123}, and Make-It-3D~\cite{tang2023make}. 
Please refer to Figure~\ref{fig:uncurated_1} and Figure~\ref{fig:uncurated_2} for visual illustrations.

% \begin{figure*}
%     \centering
%     \includegraphics[width=0.95\linewidth]{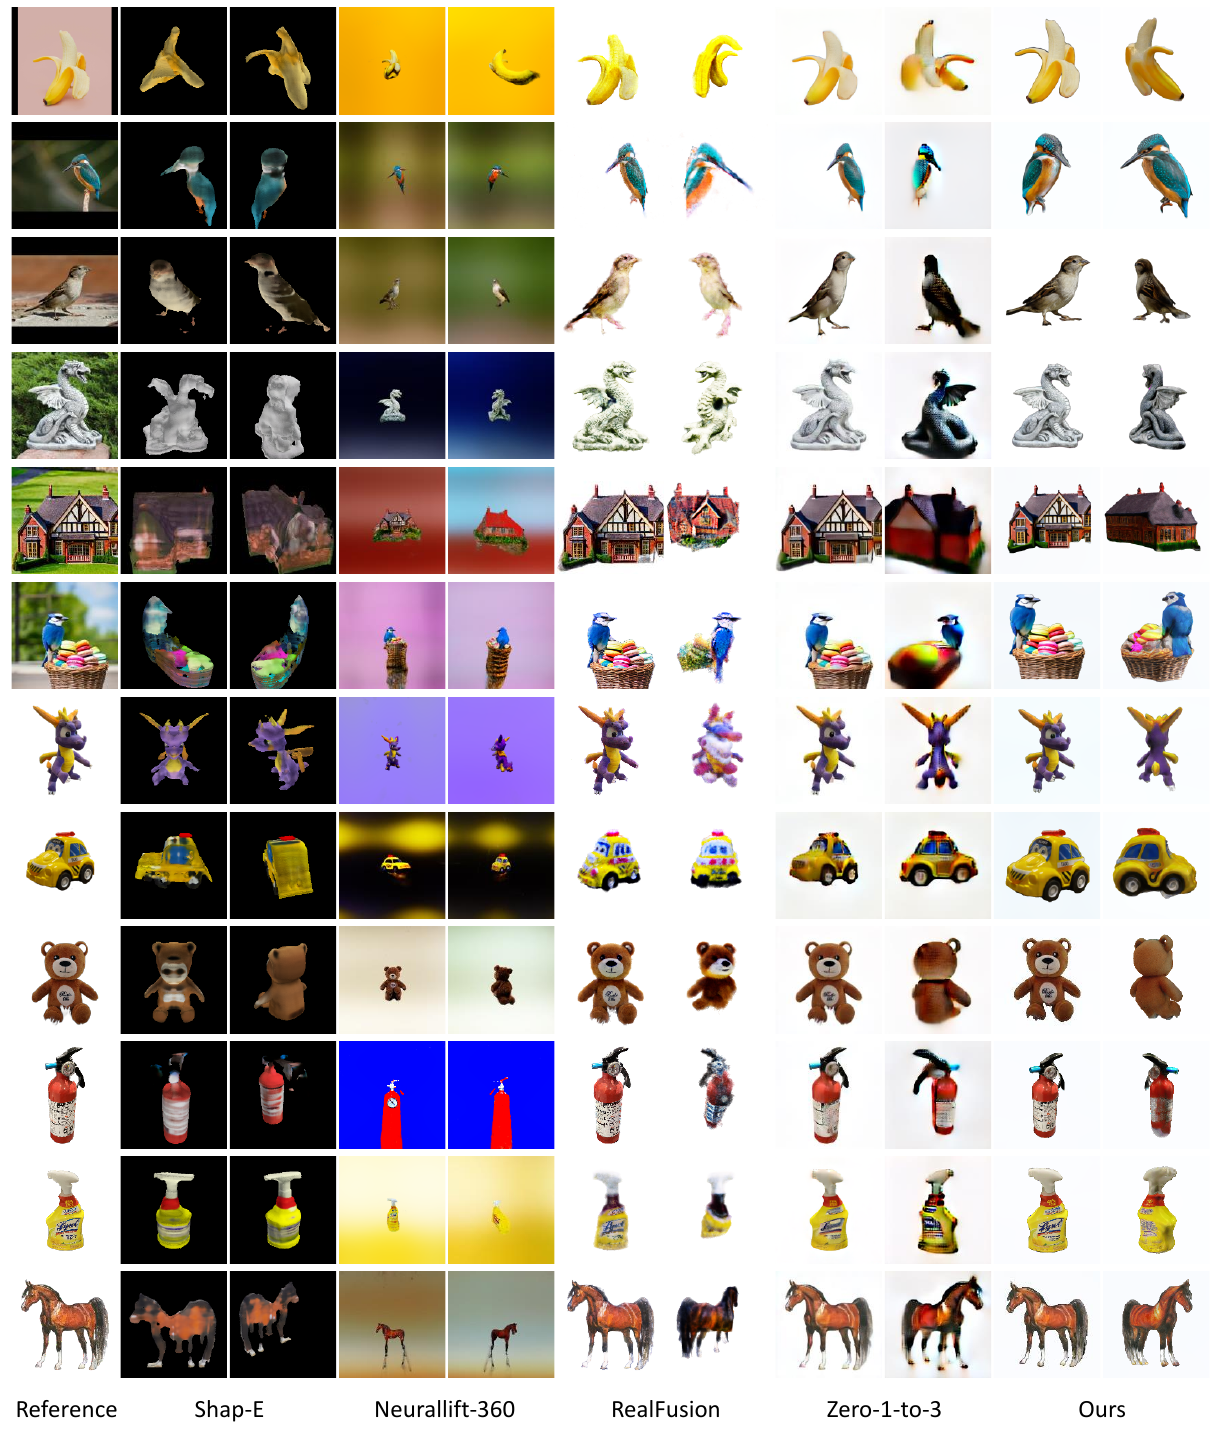}
%     \caption{\textbf{Part 1/3 of uncurated results.} We include several baselines for comparisons.}
%     \setlength{\abovecaptionskip}{-3mm}
%     \label{fig:uncurated_0}
% \end{figure*}

\begin{figure*}
    \centering
    \includegraphics[width=0.9\linewidth]{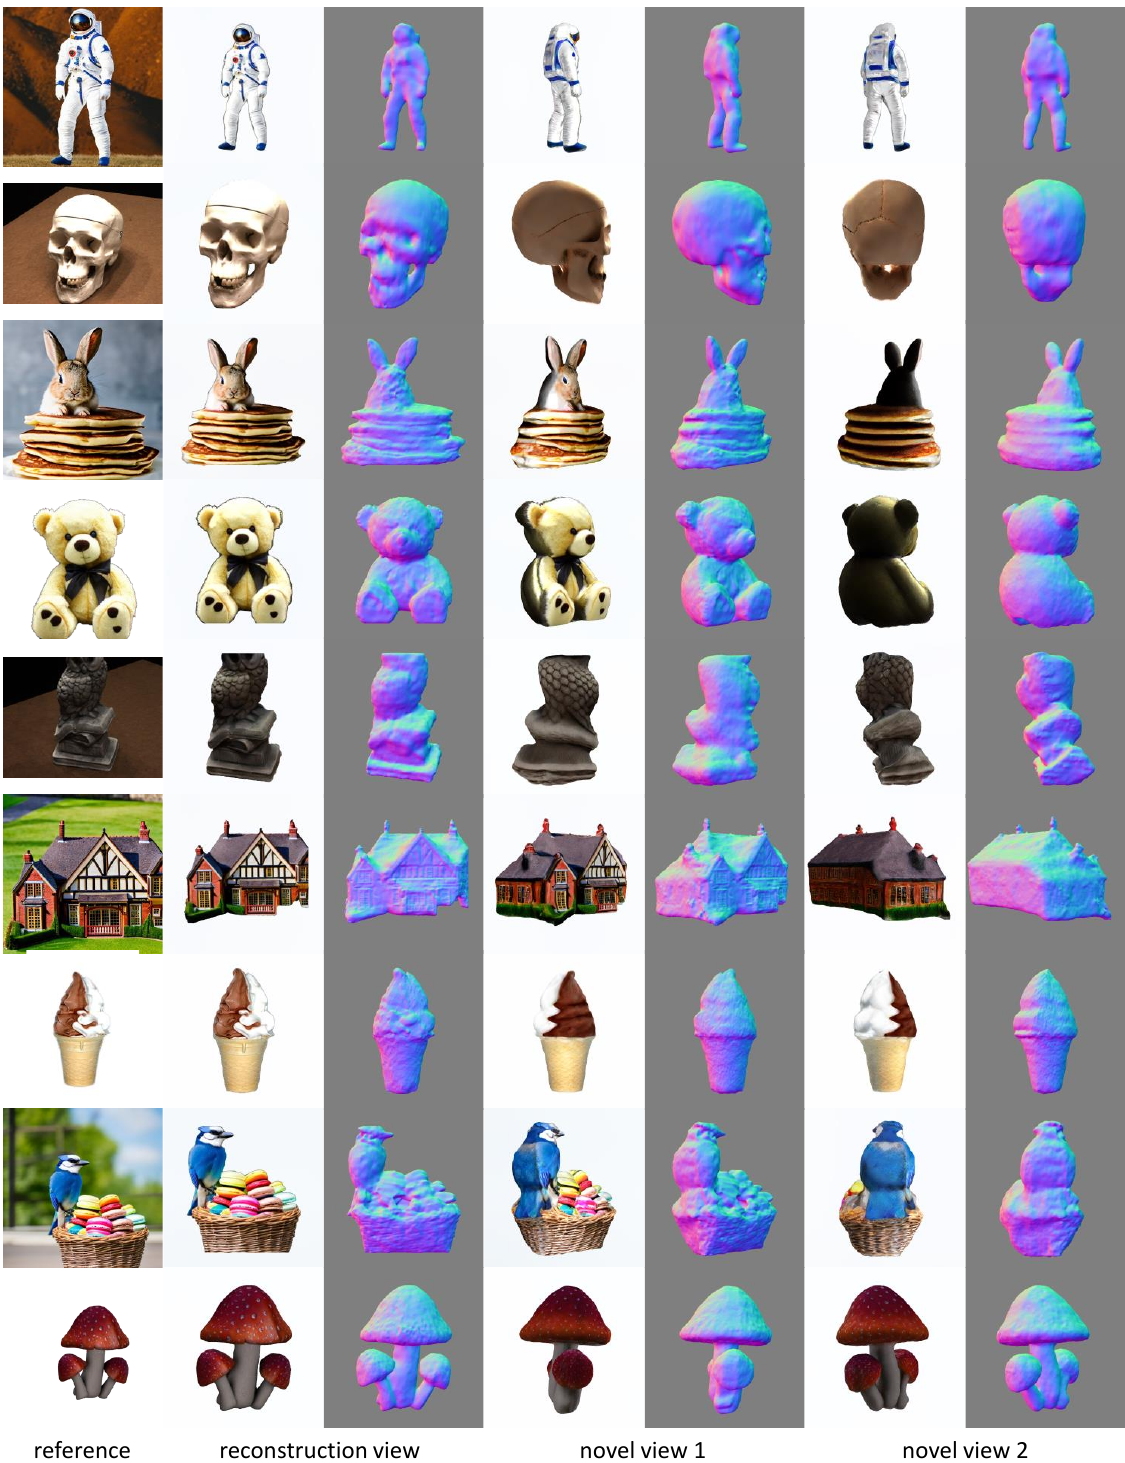}
    \caption{\textbf{Part 1/2 of uncurated results.} More views for enhanced visualization.}
    \setlength{\abovecaptionskip}{-3mm}
    \label{fig:uncurated_1}
\end{figure*}

\begin{figure*}
    \centering
    \includegraphics[width=0.9\linewidth]{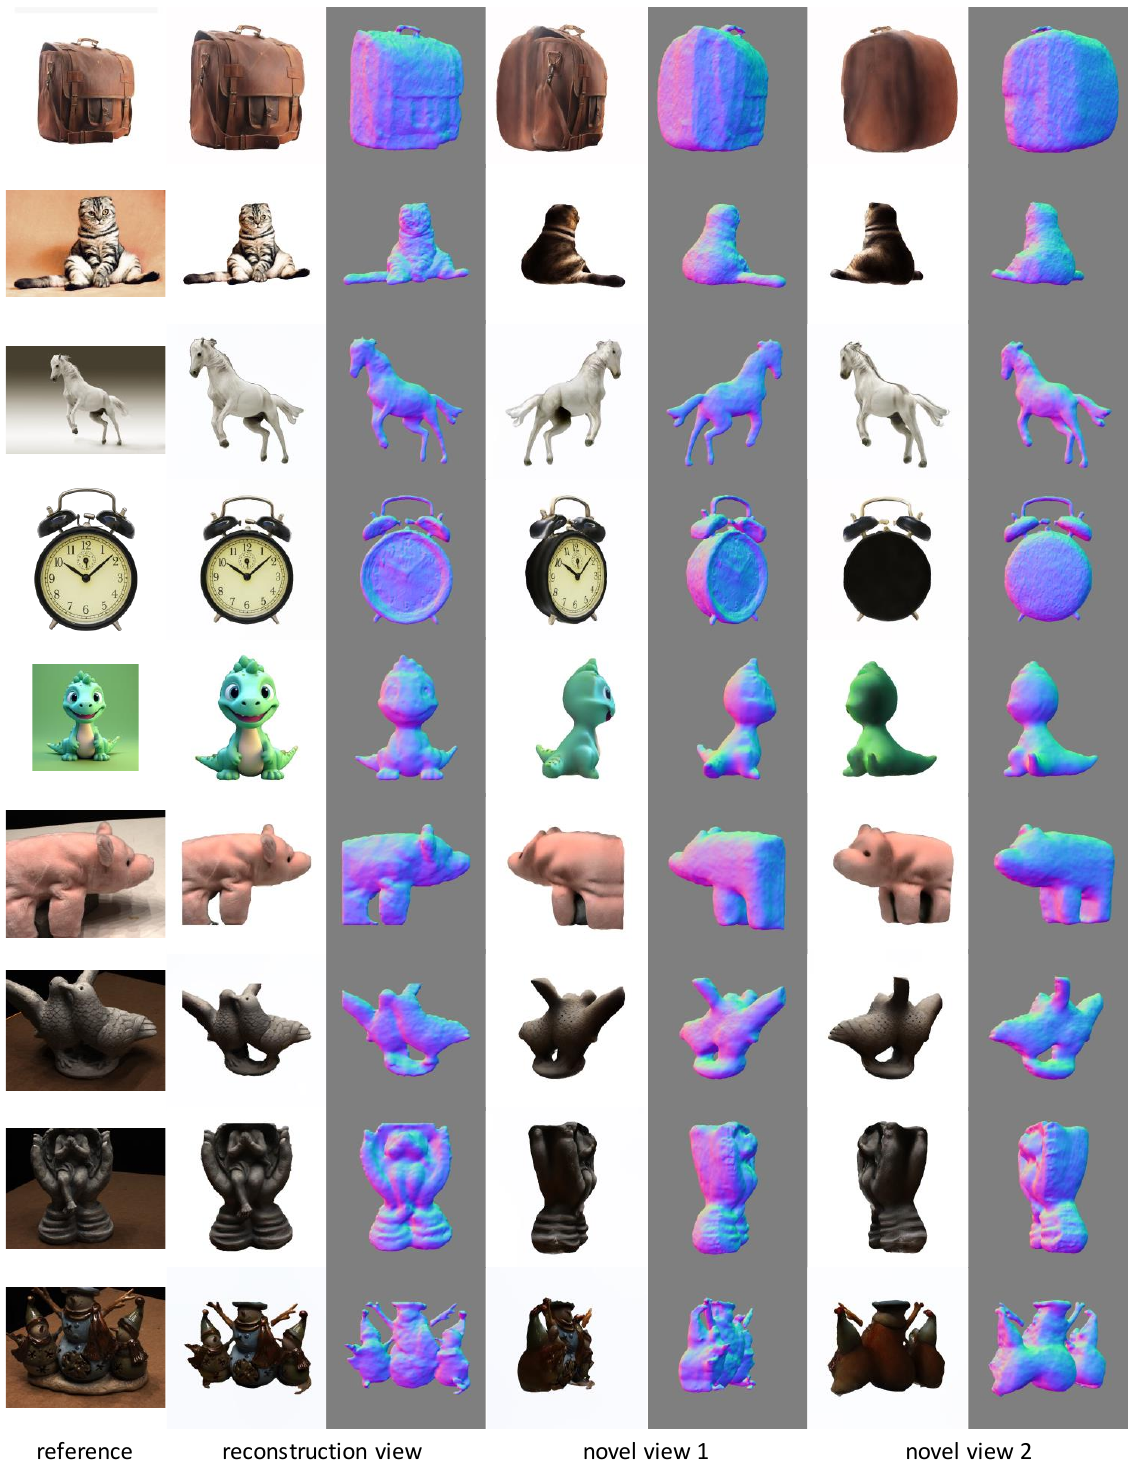}
    \caption{\textbf{Part 2/2 of uncurated results.} More views for enhanced visualization.}
    \setlength{\abovecaptionskip}{-3mm}
    \label{fig:uncurated_2}
\end{figure*}
\section{Limitations and Future Works}
The limitations of \textbf{\ourmodel} encompass various facets, opening avenues for future refinement and development:
To begin, \ourmodel~ is constructed upon pre-trained models, such as diffusion-based 2D image generation, segmentation, and derendering models. The efficacy of these underlying models profoundly influences outcomes in both generation and editing endeavors. During the generation phase, challenges arise when the geometry falls short of expectations, particularly evident when dealing with non-conventional input views, such as entire scenes as opposed to individual objects, as depicted in Figure~\ref{fig:failure_case} (a). Additionally, the utilization of a 2D generative model conditioned on normal input introduces potential quality issues in textures when the generated asset's geometry does not meet desired standards, as illustrated in Figure~\ref{fig:failure_case} (b).
To mitigate the pronounced shading artifacts introduced by 2D diffusion priors, we introduce semantic-aware regularizations. However, these remedies might not be entirely effective when the segmentation component itself is misled by prevailing shading effects, as demonstrated in Figure~\ref{fig:failure_case} (c). Lastly, the material estimation models occasionally display a tendency to predict high specular effects for regions exhibiting light colors, which may deviate from accurate representation, as showcased in Figure~\ref{fig:failure_case} (d).

Therefore, there is an opportunity to further improve the results by exploring more powerful foundational models that tackle the limitations or pursuing a better way of using existing pre-trained models.
Secondly, the current model optimizes one scene at a time, which requires approximately an hour for optimization. To better align with real-world applications, exploring a feed-forward model that is more efficient would be worth exploring.

% is designed for a single object and is not applicable for scene generation and editing. In our future work, we will try to extend the ability of \ourmodel~ from a single object to a complex scene.

\section{Copyright statement}
We have provided sources and copyright information for the images and meshes used in our paper, as detailed in Table~\ref{tab:copyright}. In addition, we have incorporated images from Make-It-3D~\cite{tang2023make} with the author's permission (Figure~\ref{fig:mi3d}). It is worth noting that the original source of these images permits their commercial use.
Any additional images and meshes not included in the table were either obtained from public datasets (DTU~\cite{aanaes2016large} and ModelNet40~\cite{wu20153d}) or generated by Stable Diffusion.

% We have excluded images from the official repository of Make-It-3D~\cite{tang2023make} that lack copyright information. The remaining images are either generated by Stable Diffusion~\cite{rombach2021highresolution} or obtained from Pixabay (refer to Figure~\ref{fig:mi3d} for specific details).
% Images for uncurated experimental results in the supplementary material are collected from official repositories of RealFusion~\cite{melaskyriazi2023realfusion}, Zero-1-to-3~\cite{liu2023zero123}, and Make-It-3D~\cite{tang2023make}. 

\begin{figure}
    \centering
    \includegraphics[width=1.0\linewidth]{figures/img_copyright/makeit3d_copyright.png}
    \caption{Copyright information of images from Make-It-3D. It is worth noting that the original source of these images permits their commercial use.}
    \label{fig:mi3d}
\end{figure}

% \newpage
% \appendix

% We give the sources of images and mesh used in this paper (See Table~\ref{tab:copyright}). Other images not included in the table are either from the DTU dataset~\cite{aanaes2016large} or generated by Stable Diffusion~\cite{rombach2021highresolution}

% Table generated by Excel2LaTeX from sheet 'Sheet1'
\begin{table*}
  \centering
  \caption{Part 1/2 of Copyright Information}
    \small
    \resizebox{.85\textwidth}{!}{
    \begin{tabular}{c|c|c}
    \toprule
    Image/Mesh & Source & License \\
    \midrule
    \multirow{2}{*}{\includegraphics[height=0.7cm]{figures/img_copyright/bag1.png}} & \multirow{2}{*}{https://pixabay.com/photos/leather-bags-duffel-bags-4379625/} & \multirow{2}{*}{free to use} \\
    & & \\
    \midrule
    \multirow{2}{*}{\includegraphics[height=0.7cm]{figures/img_copyright/bag3.png}} & \multirow{2}{*}{https://pixabay.com/photos/mens-leather-bag-8073910/} & \multirow{2}{*}{free to use} \\
    & & \\
    \midrule
    \multirow{2}{*}{\includegraphics[height=0.7cm]{figures/img_copyright/cat1.png}} & \multirow{2}{*}{https://pixabay.com/photos/cat-kitten-pets-animals-housecat-2934720/} & \multirow{2}{*}{free to use} \\
    & & \\
    \midrule
    \multirow{2}{*}{\includegraphics[height=0.7cm]{figures/img_copyright/clock1.png}} & \multirow{2}{*}{https://pixabay.com/photos/clock-alarm-clock-time-time-display-2545142/} & \multirow{2}{*}{free to use} \\
    & & \\
    \midrule
    \multirow{2}{*}{\includegraphics[height=0.7cm]{figures/img_copyright/frog3.png}} & \multirow{2}{*}{https://pixabay.com/photos/time-to-go-frog-farewell-travel-937265/} & \multirow{2}{*}{free to use} \\
    & & \\
    \midrule
    \multirow{2}{*}{\includegraphics[height=0.7cm]{figures/img_copyright/horse.png}} & \multirow{2}{*}{https://pixabay.com/illustrations/mushroom-house-fantasy-cottage-4000133/} & \multirow{2}{*}{free to use} \\
    & & \\
    \midrule
    \multirow{2}{*}{\includegraphics[height=0.7cm]{figures/img_copyright/house.png}} & \multirow{2}{*}{https://pixabay.com/illustrations/mushroom-house-fantasy-cottage-4000133/} & \multirow{2}{*}{free to use} \\
    & & \\
    \midrule
    \multirow{2}{*}{\includegraphics[height=0.7cm]{figures/img_copyright/icecream1.png}} & \multirow{2}{*}{https://pixabay.com/photos/soft-ice-cream-soft-ice-cream-cone-50845/} & \multirow{2}{*}{free to use} \\
    & & \\
    \midrule
    \multirow{2}{*}{\includegraphics[height=0.7cm]{figures/img_copyright/mushroom4.png}} & \multirow{2}{*}{https://pixabay.com/illustrations/toadstool-mushrooms-fantasy-1722288/} & \multirow{2}{*}{free to use} \\
    & & \\
    \midrule
    \multirow{2}{*}{\includegraphics[height=0.7cm]{figures/img_copyright/rose.png}} & \multirow{2}{*}{https://pixabay.com/photos/rose-flower-petals-red-rose-320868/} & \multirow{2}{*}{free to use} \\
    & & \\
    \midrule
    \multirow{2}{*}{\includegraphics[height=0.7cm]{figures/img_copyright/dinosaur2.png}} & \multirow{2}{*}{https://pixabay.com/illustrations/raptor-3d-model-render-dinosaur-5749823/} & \multirow{2}{*}{free to use} \\
    & & \\
    \midrule
    \multirow{2}{*}{\includegraphics[height=0.7cm]{figures/img_copyright/teddy2.png}} & \multirow{2}{*}{https://pixabay.com/illustrations/teddy-bear-toy-stuffed-toy-teddy-7777659/} & \multirow{2}{*}{free to use} \\
    % & & \\
    % \midrule
    % \multirow{2}{*}{\includegraphics[height=0.7cm]{figures/img_copyright/teddy.png}} & \multirow{2}{*}{Generated by Stable Diffusion} & \multirow{2}{*}{Apache License} \\
    % & & \\
    % \midrule
    % \multirow{2}{*}{\includegraphics[height=0.7cm]{figures/img_copyright/napoleon.png}} & \multirow{2}{*}{ModelNet40~\cite{wu20153d}} & \multirow{2}{*}{academic research only} \\
    % & & \\
    % \midrule
    % \multirow{2}{*}{\includegraphics[height=0.7cm]{figures/img_copyright/mushroom.png}} & \multirow{2}{*}{https://www.etsy.com/hk-en/listing/1214747045/red-mushroom-statue-colorful-painted-art} & \multirow{2}{*}{Fig~\ref{fig:mushroom_license}} \\
    & & \\
    \midrule
    \multirow{2}{*}{\includegraphics[height=0.7cm]{figures/img_copyright/rhino.png}} & \multirow{2}{*}{https://pixabay.com/photos/animal-wild-animal-rhino-africa-2765319/} & \multirow{2}{*}{free to use} \\
    & & \\
    \midrule
    \multirow{2}{*}{\includegraphics[height=0.7cm]{figures/img_copyright/white_robot.png}} & \multirow{2}{*}{https://pixabay.com/illustrations/robot-humanoid-robot-machine-6654032/} & \multirow{2}{*}{free to use} \\
    & & \\
    \midrule
    \multirow{2}{*}{\includegraphics[height=0.7cm]{figures/img_copyright/frog9.jpg}} & \multirow{2}{*}{https://pixabay.com/photos/frog-frog-prince-crown-figure-cute-1591901/} & \multirow{2}{*}{free to use} \\
    & & \\
    \midrule
    \multirow{2}{*}{\includegraphics[height=0.7cm]{figures/img_copyright/bird_1.jpg}} & \multirow{2}{*}{https://pixabay.com/photos/one-leg-birds-nature-wildlife-beak-3393491/} & \multirow{2}{*}{free to use} \\
    & & \\
    \midrule
    \multirow{2}{*}{\includegraphics[height=0.7cm]{figures/img_copyright/bird_7.jpg}} & \multirow{2}{*}{https://pixabay.com/photos/kingfisher-bird-perched-1867936/} & \multirow{2}{*}{free to use} \\
    & & \\
    \midrule
    \multirow{2}{*}{\includegraphics[height=0.7cm]{figures/img_copyright/bird2.jpg}} & \multirow{2}{*}{https://pixabay.com/illustrations/ai-generated-bird-rock-foliage-7976939/} & \multirow{2}{*}{free to use} \\
    & & \\
    % \midrule
    % \multirow{2}{*}{\includegraphics[height=0.7cm]{figures/img_copyright/sculpture1.png}} & \multirow{2}{*}{https://www.pexels.com/photo/bust-of-septimius-severus-13865689/} & \multirow{2}{*}{free to use} \\
    % & & \\
    \midrule
    \multirow{2}{*}{\includegraphics[height=0.7cm]{figures/img_copyright/mid_panda_2.png}} & \multirow{2}{*}{We generated it on Midjourney as a paid member in accordance with their agreement.} & \multirow{2}{*}{We own the asset.} \\
    & & \\
    \midrule
    \multirow{2}{*}{\includegraphics[height=0.7cm]{figures/img_copyright/mid_green_dog_1.png}} & \multirow{2}{*}{We generated it on Midjourney as a paid member in accordance with their agreement.} & \multirow{2}{*}{We own the asset.} \\
    & & \\
    \midrule
    \multirow{2}{*}{\includegraphics[height=0.7cm]{figures/img_copyright/mid_yellow_rabbit_3.png}} & \multirow{2}{*}{We generated it on Midjourney as a paid member in accordance with their agreement.} & \multirow{2}{*}{We own the asset.} \\
    & & \\
    \midrule
    \multirow{2}{*}{\includegraphics[height=0.7cm]{figures/img_copyright/mid_pink_robot2_2.png}} & \multirow{2}{*}{We generated it on Midjourney as a paid member in accordance with their agreement.} & \multirow{2}{*}{We own the asset.} \\
    & & \\
    \bottomrule
    \end{tabular}%
    }
  \label{tab:copyright1}%
\end{table*}%

\begin{table*}
  \centering
  \caption{Part 2/2 of Copyright Information}
    \small
    \resizebox{.85\textwidth}{!}{
    \begin{tabular}{c|c|c}
    \toprule
    Image/Mesh & Source & License \\
    \midrule
    \multirow{2}{*}{\includegraphics[height=0.7cm]{figures/img_copyright/mid_whitebear_1_rgba.png}} & \multirow{2}{*}{We generated it on Midjourney as a paid member in accordance with their agreement.} & \multirow{2}{*}{We own the asset.} \\
    & & \\
    \midrule
    \multirow{2}{*}{\includegraphics[height=0.7cm]{figures/img_copyright/dog3_mids_1.png}} & \multirow{2}{*}{We generated it on Midjourney as a paid member in accordance with their agreement.} & \multirow{2}{*}{We own the asset.} \\
    & & \\
    \midrule
    \multirow{2}{*}{\includegraphics[height=0.7cm]{figures/img_copyright/mouse2_mids_2.png}} & \multirow{2}{*}{We generated it on Midjourney as a paid member in accordance with their agreement.} & \multirow{2}{*}{We own the asset.} \\
    & & \\
    \bottomrule
    \end{tabular}%
    }
  \label{tab:copyright2}%
\end{table*}%
